# Supplementary material for: Deep Direct Volume Rendering: Learning Visual Feature Mappings From Exemplary Images
Source: arXiv:2106.05429 source file (2021-06-09)
Supplement: Supplementary file 1 [file 08_appendix.tex]

\appendix

\begin{needsreview}

\section{Additional Experiments}
These experiments have only been drafted or are further ideas - I just leave them here for now, but this would likely not end up in the final paper.

\subsection{Volumetric Style Transfer}\label{sec:vst}
The differentiable implementation of the whole rendering pipeline enables us to go beyond direct optimization of pixel-based similarity with the use of more advanced loss functions. Johnson et al.~\cite{Johnson2016} have successfully used a \textit{perceptual loss} to transfer the \textit{style} of an image to a target image while keeping the target's image consistent. 
%They achieved this by using a pretrained image classification network as a loss network, extracting intermediate features from that network and computing a content and style loss which they use to train a style transfer network. Their network is trained to minimize the style loss between the generated image and the style reference while at the same time keeping the content loss between generated and original image low to keep the high-level structure consistent with the original.
We can use a similar concept with our custom architectures: the style reference can be a single reference view of a volume. In practice, this can for example come from a volume rendering performed with a manually adapted high-dimensional transfer function (which requires much time to adapt) or even an image that was designed manually using 2D image editing.

To evaluate this concept, we retrain the models pretrained as in Section \ref{sec:vst} based on three different style reference images (c.f. Figure~\ref{fig:style_references}): $S_1$ is a manually selected image from a subject with high contrast between all relevant anatomical regions, thus giving a good discrimination with the manually defined intensity-based transfer function. $S_2$ is based on $S_1$, however, edited manually in an image editor to emphasize proper color separation between bones, blood vessels, kidneys and heart. $S_3$ was generated from a screenshot in an external medical volume segmentation program after semi-automatic segmentation of the CT volume and coloring the organs with a constant label color.

\begin{comment}
This is not performed yet, I'm not sure if it will still fit. the paper is getting pretty long already...
\begin{itemize}
    \item Define actual style targets
    \item write retraining code
    \item argue about partial retraining (constant feature encoder?)
    \item train all networks, report results
\end{itemize}
\end{comment}

\subsection{Illustrative Rendering}
Our DVRNet architecture has the ability to learn image-based effects by adjusting the weights of the 2D deconvolutions. We can leverage this to learn more illustrative features that do not only rely on the compositing of the samples along a single ray but instead or additionally employ more advanced compositing and post-processing in image space. For example, this can include highlighting or outlines of specific structures, depth darkening. It might even be possible to achieve importance-based rendering where specific important structures are made visible even though they would technically be hidden by occluding structures. This is related to an important visualization technique called Focus and Context visualization (F+C), where the focus structure is shown with high detail while surrounding important tissues (such as for example the skin surface or bone structure) are still made visible for context where appropriate.

We can generate a test data set by combining multiple renderings of our volumes, leveraging the labels of our data set:
We first render the volume with a conventional transfer function to achieve a surface rendering which forms the context layer. We generate secondary images with a separate raymarching that only renders the labeled focus structures with a specific transfer function. We can then create an illustrative rendering by combining these two images, compositing the focus structures on top of the context.

These images can then be used in our end-to-end training. As an input to our rendering models, we test two variants: For one, we provide the input grayscale volume as well as the binary label map as a two-channel input to the models such that they can leverage the existing labels. This evaluates the architectures' capability to learn the rendering transformation taking the labels into account.
As a second, more challenging case, we only provide the grayscale input image. In this case, the models have to learn to detect the relevant structures in addition to the rendering task itself.

\begin{comment}
\begin{itemize}
    \item Pretrain volume encoder on segmentation task?
    \item train colorization/rendering, only train head of network
\end{itemize}
\end{comment}

\subsection{Performance Analysis}
\begin{comment}
This might need a (short) description of the implementation details of the renderer (i.e. image-slice compositing as opposed to shader-based implementation). Discuss shader-based difference here (no need for storing the whole render buffer here).

A detailed analysis of the performance characteristics of each network. Define toy task (small\_heart? synthetic?) and analyze performance with respect to Volume Size, Sampling Rate, rendered image size
\begin{enumerate}
    \item Memory Scaling (train, inference)
    \item Training time scaling
    \item Rendering time scaling
\end{enumerate}
\end{comment}

\subsection{Multi-Modal}
\begin{comment}
Not even sure what/how to do it, but it would be a really cool addition to show our method has benefits in multimodal volume rendering.
\end{comment}

\subsection{Introspection}
\begin{comment}
Color mapping from feature space (PCA) to color
\end{comment}

\end{needsreview}
